# Supplementary material for: A Novel Architecture Slimming Method for Network Pruning and Knowledge Distillation
Source: arXiv:2202.10461 source file (2022-02-21)
Supplement: Supplementary file 1 [file 6.Appendix.tex]

\section{Appendix}
\label{sec:appendix}
